# Supplementary material for: Divide-and-Conquer Posterior Sampling for Denoising Diffusion Priors
Source: arXiv:2403.11407 source file (2024-11-11)
Supplement: Supplementary file 1 [file gibbs_sampler.tex]

\subsection{Approximate Gibbs sampler}
    \label{subsec:gibbs}
We now detail how one can use an approximate Gibbs sampler to sample from $\bwmarg{\tstep{\ell+1}}{}[\obs, \ell]$. We assume that $\eta = 1$ for convenience. By \eqref{eq:ipot} and \eqref{eq:ibwtrans}, $\bwmarg{\tstep{\ell+1}}{}[y,\ell]$ is the marginal of the joint distribution
\begin{equation*}
\bwmarg{\tstep{\ell}, \tstep{\ell+1}}{\rmd (x_\tstep{\ell}, x_\tstep{\ell+1})}[\obs, \ell] \propto \pot{\tstep{\ell}}{\obs}{x_\tstep{\ell}} \, \bwmarg{\tstep{\ell}, \tstep{\ell+1}}{\rmd (x_\tstep{\ell}, x_\tstep{\ell+1})} \eqsp.
\end{equation*}
Therefore, we can use Gibbs sampling to sample from it. Indeed, under this joint distribution, the law of $X_\tstep{\ell} | X_\tstep{\ell+1} = x_\tstep{\ell+1}$ is given by
$$
\abwker{\tstep{\ell}|\tstep{\ell+1}}{x_\tstep{\ell+1}}{\rmd x_\tstep{\ell}}[\obs, \ell] \propto \ipot{\tstep{\ell}}{\obs}{x_\tstep{\ell}} \abwker{\tstep{\ell}|\tstep{\ell+1}}{x_\tstep{\ell+1}}{\rmd x_\tstep{\ell}} \eqsp,
$$
and we may, as previously, approximate it using the Gaussian approximation \eqref{eq:gauss_approx_ddim} of $\abwker{\tstep{\ell}|\tstep{\ell+1}}{x_\tstep{\ell+1}}{\rmd x_\tstep{\ell}}$. The resulting approximation, which we denote by $\aabwker{\tstep{\ell}|\tstep{\ell+1}}{x_\tstep{\ell+1}}{\cdot}[\obs, \ell]$, can then be computed in a closed form since $\pot{\tstep{\ell}}{\obs}{}$ is a Gaussian distribution whose mean is linear in $x_\tstep{\ell}$.

We turn to the second conditional $X_\tstep{\ell+1} | X_\tstep{\ell} = x_\tstep{\ell}$, which is given by
$$
\abwker{\tstep{\ell+1}|\tstep{\ell}}{x_\tstep{\ell}}{\rmd x_\tstep{\ell+1}} \propto \bwmarg{\tstep{\ell+1}}{\rmd x_\tstep{\ell+1}} \abwker{\tstep{\ell}|\tstep{\ell}+1}{x_\tstep{\ell+1}}{x_\tstep{\ell}}.
$$
Assuming that $\abwker{\tstep{\ell}|\tstep{\ell+1}}{x_{\tstep{\ell+1}}}{\rmd x_{\tstep{\ell}}}$ and $\bwmarg{\tstep{\ell}}{}$ are approximately equal to $ \fwtrans{\tstep{\ell}|\tstep{\ell+1}}{x_\tstep{\ell+1}}{\rmd x_{\tstep{\ell}}}[\eta]$ and $\fwmarg{\tstep{\ell}}{}$, respectively, it holds that  $\abwker{\tstep{\ell+1}|\tstep{\ell}}{x_\tstep{\ell}}{\rmd x_{\tstep{\ell + 1}}}$ is approximately equal to $\fwtrans{\tstep{\ell+1}|\tstep{\ell}}{x_\tstep{\ell}}{\rmd x_{\tstep{\ell + 1}}}$, which allows us to draw an approximate sample by simply using the forward transition \eqref{eq:fwd_onestep}.
% $$
We further detail both steps below.

\eric{strange "Conditional"...}
\paragraph{Conditional $X_\tstep{\ell+1} | X_\tstep{\ell}$.}
First, we assume that $\eta = 1$, since in this case we have that \citep[see][Section 4.1]{song2021denoising}
$$
    \rbwker{m|0, m+1}{x_0, x_{m+1}}{\rmd x_m}[\eta] = \frac{\fwtrans{m|0}{x_0}{\rmd x_m} \fwtrans{m+1|m}{x_m}{x_{m+1}}}{\fwtrans{m+1|0}{x_{0}}{x_{m+1}}} \eqsp,
$$
where $\fwtrans{m+1|m}{x_m}{\rmd x_{m + 1}}$ is the Markov transition associated to \eqref{eq:fwd_onestep}. Using \eqref{eq:inference_bw} and the definition of the backward kernel $\rbwker{0|m+1}{x_{m+1}}{}$ yields
\begin{equation}
    \label{eq:etaone_bw_def}
\rbwker{m|m+1}{x_{m+1}}{\rmd x_m}[\eta] = \frac{\fwmarg{m}{\rmd x_m} \fwtrans{m+1|m}{x_m}{x_{m+1}}}{\fwmarg{m+1}{x_{m+1}}} \eqsp.
\end{equation}
Hence, assuming that $\bwmarg{\tstep{\ell}}{}$ is approximately equal to $\fwmarg{\tstep{\ell}}{}$, we find that
$$
\bwmarg{\tstep{\ell}}{\rmd x_\tstep{\ell}} \fwtrans{\tstep{\ell+1}|\tstep{\ell}}{x_\tstep{\ell}}{\rmd x_{m+1}} \approx \bwmarg{\tstep{\ell+1}}{\rmd x_\tstep{\ell+1}} \abwker{\tstep{\ell}|\tstep{\ell+1}}{x_\tstep{\ell+1}}{\rmd x_\tstep{\ell}} \eqsp,
$$
and we may thus use the forward transition kernel $\rbwker{\tstep{\ell+1}|\tstep{\ell}}{\tstep{\ell}}{\rmd x_\tstep{\ell+1}}$ as the reversal of $\abwker{\tstep{\ell}|\tstep{\ell+1}}{x_\tstep{\ell+1}}{\rmd x_\tstep{\ell}}$.
\paragraph{Conditional $X_\tstep{\ell} | X_\tstep{\ell+1}$.}
We remind the reader that by \eqref{eq:ipot} and \eqref{eq:ibwtrans}, $\bwmarg{\tstep{\ell+1}}{}[y,\ell]$ is the marginal of the joint distribution
\begin{equation*}
\bwmarg{\tstep{\ell}, \tstep{\ell+1}}{\rmd (x_\tstep{\ell}, x_\tstep{\ell+1})}[\obs] \propto \pot{\tstep{\ell}}{\obs}{x_\tstep{\ell}} \, \bwmarg{\tstep{\ell}, \tstep{\ell+1}}{\rmd (x_\tstep{\ell}, x_\tstep{\ell+1})} \eqsp,
\end{equation*}
and under this joint distribution, the law of $X_\tstep{\ell} | X_\tstep{\ell+1} = x_\tstep{\ell+1}$ is
$$
\abwker{\tstep{\ell}|\tstep{\ell+1}}{x_\tstep{\ell+1}}{\rmd x_\tstep{\ell}}[\obs, \ell] \propto \ipot{\tstep{\ell}}{\obs}{x_\tstep{\ell}} \, \abwker{\tstep{\ell}|\tstep{\ell+1}}{x_\tstep{\ell+1}}{\rmd x_\tstep{\ell}} \eqsp.
$$
We approximate this distribution by $\aabwker{\tstep{\ell}|\tstep{\ell+1}}{x_\tstep{\ell+1}}{\rmd x_{\tstep{\ell}}}[\obs, \ell]$ using the Gaussian approximation \eqref{eq:gauss_approx_ddim} of $\abwker{\tstep{\ell}|\tstep{\ell+1}}{x_\tstep{\ell+1}}{\rmd x_\tstep{\ell}}$, \emph{i.e.},
\begin{equation}
    \label{eq:gibbs_taul_giv_taulnext}
\aabwker{\tstep{\ell}|\tstep{\ell+1}}{x_\tstep{\ell+1}}{\rmd x_\tstep{\ell}}[\obs, \ell] \propto \ipot{\tstep{\ell}}{\obs}{x_\tstep{\ell}} \, \aabwker{\tstep{\ell}|\tstep{\ell+1}}{x_\tstep{\ell+1}}{\rmd x_\tstep{\ell}} \eqsp.
\end{equation}
Using \citep[Eq. 2.116]{bishop2006pattern} and definitions \eqref{eq:ipot_def} \eqref{eq:gauss_approx_ddim}, we obtain that
\begin{equation}
    \label{eq:cbwker_taul_giv_taulnext}
\aabwker{\tstep{\ell}|\tstep{\ell+1}}{x_\tstep{\ell+1}}{x_\tstep{\ell}}[\obs, \ell] = \normpdf\left(x_\tstep{\ell}; \Sigma^{\obs, \ell} _{\tstep{\ell+1}} \left(   \frac{A^\intercal \obs}{\sigma^2 _{\obs, \ell}} + \frac{\muDDIM{\tstep{\ell}|\tstep{\ell+1}}(x_\tstep{\ell+1})}{\sigma^2 _{\tstep{\ell}|\tstep{\ell+1}}}  \right) ,\Sigma^{\obs, \ell} _{\tstep{\ell+1}}\right) \eqsp,
\end{equation}
where
\begin{equation}
    \label{eq:cov_mat}
\Sigma^{\obs, \ell} _{\tstep{\ell+1}} \eqdef \left( \frac{1}{\sigma^2 _{\tstep{\ell}|\tstep{\ell+1}}} \Id_\dimx + \frac{1}{\sigma^2 _{\obs, \ell}} \bfA^\intercal \bfA \right)^{-1} \eqsp.
\end{equation}
\begin{algorithm}
    \caption{One step of approximate Gibbs sampler with matrix inversion}
    \begin{algorithmic}[1]
        \STATE {\bfseries Input:} Observation $\obs$, number $M$ of Gibbs steps, initial sample $X^{\obs, \ell} _{\tstep{\ell+1}}$
        \STATE {\bfseries Output:} $X^{\obs, \ell} _{\tstep{\ell+1}, M+1}$
        \STATE Initial sample $X^{\obs, \ell} _{\tstep{\ell+1}, 1} = X^{\obs, \ell} _{\tstep{\ell+1}}$;
        \FOR{$i = 1$ {\bfseries to} $M$}
            \STATE $X^{\obs, \ell} _{\tstep{\ell}, i} \sim \aabwker{\tstep{\ell}|\tstep{\ell+1}}{X^{\obs, \ell} _{\tstep{\ell+1}, i}}{\cdot}[\obs, \ell]$ following \eqref{eq:cbwker_taul_giv_taulnext};
            \STATE $X^{\obs, \ell} _{\tstep{\ell+1},i+1} = \sqrt{\acp{\tstep{\ell+1}} / \acp{\tstep{\ell}}} X^{\obs, \ell} _{\tstep{\ell}, i} + \sqrt{1 - \acp{\tstep{\ell+1}} / \acp{\tstep{\ell}}} Z_i$, where $Z_i \sim \gauss(\zero_\dimx, \Id_\dimx)$;
        \ENDFOR
    \end{algorithmic}
    \label{algo:gibbs_matrix_inv}
   \end{algorithm}
   \paragraph{\textsc{RePaint}.} The approximate Gibbs sampler perspective allows us to re-frame the RePaint algorithm of \citet{lugmayr2022repaint} as a special case of our framework. For the sake of simplicity, we assume that $\bfA$ is rectangular unit diagonal, \emph{i.e.}, that we only observe the first $\dimobs$ coordinates of a sample from the prior. We denote by $\overline{X}$ the first $\dimobs$ coordinates of $X \in \rset^\dimx$ and by $\underline{X}$ the remaining ones. Then, step~5 of \Cref{algo:gibbs_matrix_inv} is equivalent to setting $X^\obs _{\tstep{\ell}, i} = [ \overline{X}^{\obs, \ell} _{\tstep{\ell+1}, i},  \underline{X}^{\obs, \ell} _{\tstep{\ell+1}, i}]$, where
   \begin{align*}
        \overline{X}^{\obs, \ell} _{\tstep{\ell}, i} & = \frac{\sigma^2 _{\tstep{\ell}|\tstep{\ell+1}}}{\sigma^2 _{\obs, \ell} + \sigma^2 _{\tstep{\ell}|\tstep{\ell+1}}} \obs_{\tstep{\ell}} + \frac{\sigma^2 _{\obs, \ell}}{\sigma^2 _{\obs, \ell} + \sigma^2 _{\tstep{\ell}|\tstep{\ell+1}}} \overline{\muDDIM{\tstep{\ell}|\tstep{\ell+1}}(X^\obs _{\tstep{\ell+1}, i})} +  \frac{\sigma^2 _{\obs, \ell} \sigma^2 _{\tstep{\ell}|\tstep{\ell+1}}}{\sigma^2 _{\obs, \ell} + \sigma^2 _{\tstep{\ell}|\tstep{\ell+1}}} \overline{Z}_i \eqsp,\\
        \underline{X}^{\obs, \ell} _{\tstep{\ell}, i} & =  \underline{\muDDIM{\tstep{\ell}|\tstep{\ell+1}}(X^\obs _{\tstep{\ell+1}, i})} +  \sigma^2 _{\tstep{\ell}|\tstep{\ell+1}} \underline{Z}_i.
   \end{align*}
   Thus, if we choose $\tauks = \last$, implying that $\tstep{\ell} = \ell$, we recover a generalization of the RePaint algorithm. In the specific case of an inverse problem with $\stdobs = 0$, we can, setting for all $\ell$ $\sigma _{\obs, \ell} = 0$ and $\obs_\ell = \sqrt{\acp{\ell}} \, \obs + \sqrt{1 - \acp{\ell}} Z_\ell$ and $Z_\ell$ are i.i.d. standard Gaussian samples, recover the Algorithm 1 in \citet{lugmayr2022repaint}.
\paragraph{Variational approximation.} When this matrix inversion is prohibitively expensive, which is typically the case in very large dimensions, we propose the use of a diagonal Gaussian variational approximation of \eqref{eq:gibbs_taul_giv_taulnext}. This is done by solving %minimizing
%over $\dgvf$
$$
   \argmin_{\vbwker{\tstep{\ell}|\tstep{\ell+1}}{x_{\ell+1}}{\cdot}[\obs, \ell] \in \dgvf} \kldivergence{\vbwker{\tstep{\ell}|\tstep{\ell+1}}{x_{\ell+1}}{\cdot}[\obs, \ell]}{\aabwker{\tstep{\ell}|\tstep{\ell+1}}{x_{\ell+1}}{\cdot}[\obs, \ell]} \eqsp,
$$
where the KL can be computed in a closed form. Indeed, this is equivalent to the following minimization problem
$$
    \argmin_{(\vmu_{\tstep{\ell|\tstep{\ell+1}}}, s_{\tstep{\ell}|\tstep{\ell+1}}) \in \rset^\dimx \times \rset^\dimx} \mathcal{L}^{\obs, \ell} _{\tstep{\ell} | \tstep{\ell+1}}(\vmu_{\tstep{\ell} | \tstep{\ell+1}}, s_{\tstep{\ell} | \tstep{\ell+1}}; x_{\tstep{\ell+1}}),
$$
where
\begin{multline*}
\mathcal{L}^{\obs, \ell} _{\tstep{\ell} | \tstep{\ell+1}}(\vmu_{\tstep{\ell} | \tstep{\ell+1}}, s_{\tstep{\ell} | \tstep{\ell+1}}; x_{\tstep{\ell+1}}) \eqdef
 \frac{1}{\sigma^2 _{\obs, \ell}}\| \sqrt{\acp{\tstep{\ell}}} \obs - \bfA \vmu_{\tstep{\ell}|\tstep{\ell+1}} \|^2 + \frac{1}{\sigma^2 _{\obs, \ell}}\trace(\bfA(\Id_\dimx \rme^{s_{\tstep{\ell} | \tstep{\ell+1}}}) \bfA^\intercal) \\
 + \frac{1}{2 \sigma^2 _{\tstep{\ell}|\tstep{\ell+1}}}\| \vmu_{\tstep{\ell}|\tstep{\ell+1}} - \muDDIM{\tstep{\ell}|\tstep{\ell+1}}(x_{\tstep{\ell+1}})\|^2 - \frac{1}{2}\sum_{i = 1}^\dimx \parenthese{s_{\tstep{\ell}|\tstep{\ell+1}, i} - \frac{\rme^{s_{\tstep{\ell}|\tstep{\ell+1}, i}}}{\sigma^2 _{\tstep{\ell}|\tstep{\ell+1}}}} \eqsp.
\end{multline*}
We optimize this loss using SGD, and the complete algorithm is summarized in \Cref{algo:gibbs_vi}.
\begin{algorithm}[H]
    \caption{One step of the approximate Gibbs sampler with diagonal Gaussian approximation}
    \begin{algorithmic}[1]
        \STATE {\bfseries Input:} Observation $\obs$, number $M$ of Gibbs steps, initial sample $X^{\obs, \ell} _{\tstep{\ell+1}}$, number $V$ of VI steps
        \STATE {\bfseries Output:} $X^{\obs, \ell} _{\tstep{\ell+1}, M+1}$
        \STATE Initial sample $X^{\obs, \ell} _{\tstep{\ell+1}, 1} = X^{\obs, \ell} _{\tstep{\ell+1}}$;
        \FOR{$i = 1$ {\bfseries to} $M$}
            \STATE Set $\vmu_1 = \muDDIM{\tstep{\ell}|\tstep{\ell+1}}$, $s_1 = \log \sigma^2 _{\tstep{\ell}|\tstep{\ell+1}} \mathbf{1}_\dimx$;
            \FOR{$j = 1$ {\bfseries to} $V$}
                \STATE \textcolor{blue}{\textbf{\scriptsize // $\predx{\tstep{\ell+1}}(X^{\obs, \ell} _{\tstep{\ell+1}, i})$ \texttt{is  computed only once}.}}
                \STATE $\vmu_{j+1} = \vmu_j - \| \nabla_\mu \mathcal{L}^{\obs, \ell} _{\tstep{\ell}|\tstep{\ell}+1}(\vmu_j, s_j; X^{\obs, \ell} _{\tstep{\ell+1}, i})\|^{-1}\nabla_\mu \mathcal{L}^{\obs, \ell} _{\tstep{\ell}|\tstep{\ell}+1}(\vmu_j, s_j; X^{\obs, \ell} _{\tstep{\ell+1}, i})$;
                \STATE $s_{j+1} = s_j -  \| \nabla_s \mathcal{L}^{\obs, \ell} _{\tstep{\ell}|\tstep{\ell}+1}(\vmu_j, s_j; X^{\obs, \ell} _{\tstep{\ell+1}, i})\|^{-1} \nabla_s \mathcal{L}^{\obs, \ell} _{\tstep{\ell}|\tstep{\ell}+1}(\vmu_j, s_j; X^{\obs, \ell} _{\tstep{\ell+1}, i})$;
            \ENDFOR
            \STATE $X^{\obs, \ell} _{\tstep{\ell}, i} \sim \gauss(\vmu_{V+1}, \Id_\dimx \rme^{s_{V+1} / 2})$;
            \STATE $X^{\obs, \ell} _{\tstep{\ell+1},i+1} = \sqrt{\acp{\tstep{\ell+1}} / \acp{\tstep{\ell}}} X^{\obs, \ell} _{\tstep{\ell}, i} + \sqrt{1 - \acp{\tstep{\ell+1}} / \acp{\tstep{\ell}}} Z_i$, where $Z_i \sim \gauss(\zero_\dimx, \Id_\dimx)$;
        \ENDFOR
    \end{algorithmic}
    \label{algo:gibbs_vi}
   \end{algorithm}
